# Supplementary material for: Sensing-Constrained LQG Control
Source: arXiv:1709.08826 source file (2020-05-14)
Supplement: Supplementary file 1 [file Deprecated_Appendix_Vassilis.tex]

%!TEX root = ../main.tex

\section*{Appendix A: Separation theorem \& certainty equivalence principle in Problem~\ref{prob:LQG}}

We prove that a separation theorem --between the controller design and the sensor selection-- as well as the certainty equivalence principle 
hold for the sensing-constrained Problem~\ref{prob:LQG}.

\begin{mytheorem}[Separation of control and sensor design]\label{th:LQG_closed}
Let the sensor set $\calS^\star$ and the controllers $u_1^\star, u_2^\star, \ldots, u_T^\star$ be a solution to the sensing-constrained~Problem~\ref{prob:LQG}. Then, $\calS^\star$  and $u_1^\star, u_2^\star, \ldots, u_T^\star$ can be computed in cascade as follows: 
\begin{align}
\calS^\star &\in \argmin_{\calS \subseteq \calV, |\calS|\leq k}\sum_{t=1}^T\text{tr}[\Theta_t\Sigma\att{t}{t}(\calS)],\label{eq:opt_sensors}\\
u_t^\star&=K_t\hat{x}_{t,\calS^\star}, \quad t=1,\ldots,T\label{eq:opt_control}
\end{align}
\LC{need to define/recall expression of $\hat{x}_{t,\calS^\star}$}
where the matrices $\Theta_t$, $K_t$, and $\Sigma\att{t}{t}$ are computed as follows:
\begin{itemize}
\item for $t \in \{1,2,\ldots, T\}$, the matrices $\Theta_t$ and $K_t$ are the solution of the backward Riccati recursion
\beal\label{eq:control_riccati}
S_t &= Q_t + N_{t+1}, \\
N_t &= A_t\tran (S_t\inv+B_tR_t\inv B_t\tran)\inv A_t, \\
%\quad\mbox{ } = A_t\tran (S_t - S_t B_t M_t\inv B_t\tran S_t) A_t\\
%\quad\mbox{ } =A_t\tran S_t A_t-\Theta_t\\ 
M_t &= B_t\tran S_t B_t + R_t, \\ 
K_t &= - M_t\inv B_t\tran S_t A_t, \\ 
\Theta_t &= K_t\tran M_t K_t,
\eeal
with boundary condition $N_{T+1}=0$;
\item for $t \in \{1,2,\ldots, T\}$, and any sensor set $\calS$, the matrix $\Sigma\att{t}{t}(\calS)$ is the solution of the Kalman filtering recursion
\beq\label{eq:covariance_riccati}
\begin{array}{rcl}
\Sigma\att{t}{t}(\calS) \!\!&\!\!=\!\!&\!\![ 
\Sigma\att{t}{t-1}(\calS)\inv + C_t(\calS)\tran V_t(\calS)\inv C_t(\calS)]\inv\!\!,\\
\Sigma\att{t}{t-1}(\calS) \!\!&\!\!=\!\!&\!\! A_{t-1} \Sigma\att{t-1}{t-1}(\calS) A_{t-1}\tran + W_{t-1},
\end{array}
\eeq
with boundary condition the $\Sigma\att{1}{1}(\calS)=\Sigma\att{1}{1}$. 
\end{itemize}
\end{mytheorem}

Theorem~\ref{th:LQG_closed} implies the separation between the controller design and the sensor selection in Problem~\ref{prob:LQG}, since eq.~\eqref{eq:opt_control} implies that the optimal controllers for Problem~\ref{prob:LQG} are decided independently of the optimal  sensor set: the matrices $K_1, K_2$, $\ldots, K_T$ are independent of the selected sensor set. 
%Similarly, the 
%optimal sensor selection in~\eqref{eq:opt_sensors} can be done independently on the control actions 
%$u_1^\star, u_2^\star, \ldots, u_T^\star$.

\LC{I would make this a small corollary/remark}
Theorem~\ref{th:LQG_closed} implies the certainty equivalence principle since the control gain matrices $K_1, K_2, \ldots, K_T$
are the same control gain matrices that make the control policies $(K_1x_1$, $K_1x_2,\ldots, K_T x_T)$ optimal for the perfect state information version of Problem~\ref{prob:LQG}, where at any time $t \in \until{T}$ the state $x_t$ is known~\cite[Chapter~4]{bertsekas2005dynamic}.

The proof of Theorem~\ref{th:LQG_closed} follows from the following lemma.

\begin{mylemma}\label{lem:LQG_closed}
For any sensor set $\calS\subseteq\calV$, and control policies $u_1 \in \mathbb{R}^{m_1}, u_2 \in \mathbb{R}^{m_2}, \ldots, u_T \in \mathbb{R}^{m_T}$, let $J(\calS, u_1,u_2,\ldots,$ $u_T)$ be the cost function in Problem~\ref{prob:LQG}, i.e.,
\LC{from the following expression is unclear how the right hand side depends on S}
\begin{equation*}
J(\calS, u_1,u_2,\ldots,u_T)=\sum_{t=1}^{T}\mathbb{E}(x\at{t+1}\tran Q_t x\at{t+1}+u_t\tran R_t u_t).
\end{equation*}

Consider any sensor set $\calS \subseteq \calV$, and let $p_\calS$  be the vector of control policies $(K_1\hat{x}_{1,\calS}, K_2\hat{x}_{2,\calS}, \ldots, K_T\hat{x}_{T,\calS})$.
\begin{align}
& p_\calS \in \arg \min_{u_t \in \mathbb{R}^{m_t}}J(\calS, u_1, u_2, \ldots, u_T);\label{eq:lem:opt_control}\\
& J(\calS, p_\calS)=
\mathbb{E}(x_1\tran N_1x_1)+\nonumber\\
&\qquad\qquad\hspace{0.8em}\sum_{t=1}^T\left\{\text{tr}[\Theta_t\Sigma\att{t}{t}(\calS)]+\trace{W_tS_t}\right\}\label{eq:lem:opt_sensors}.
\end{align}
\end{mylemma}
\begin{proof}[Proof of Lemma~\ref{lem:LQG_closed}]
Let
\begin{itemize}
\item for any matrix $M$, and vector $v$ of appropriate dimension, $\|v\|_M^2=v\tran M v$;
\item for any sensor set $\calS\subseteq\calV$, and control policies $u_1 \in \mathbb{R}^{m_1}, u_2 \in \mathbb{R}^{m_2}, \ldots, u_T \in \mathbb{R}^{m_T}$, $J_t(\calS, u_t,u_{t+1},\ldots,u_T)$ to be Problem~\ref{prob:LQG}'s LQG cost function from time $t$ up to time $T$, i.e.,
\begin{equation*}
J_t(\calS, u_{t}, u_{t+1}, \ldots, u_T)=\sum_{k=t}^T\mathbb{E}(\|x_{k+1}\|^2_{Q_t}+\|u_{k,\calS}\|^2_{R_t}).
\end{equation*}
\item $J_t^\star(\calS)=\min_{u_k \in \mathbb{R}^{m_k}}J_t(\calS, u_{t}, u_{t+1}, \ldots, u_T).$  
\end{itemize} 

We complete the proof inductively.  In particular, we first prove Lemma~\ref{lem:LQG_closed} for $t=T$, and then for any other $t\in \{1,2,\ldots, T-1\}$. To this end, we use the following observation: given any sensor set $\calS$, and any time $t \in \{1,2,\ldots, T\}$, \beal\label{eq:LQG_closed_reduction_step_1}
J_t^\star(\calS)=\min_{u_t \in \mathbb{R}^{m_t}} \left[ \mathbb{E}(\|x_{t+1}\|^2_{Q_t}+\|u_t\|^2_{R_t})+ J_{t+1}^\star(\calS)\right],
\eeal 
with boundary condition the $J_{T+1}^\star(\calS)=0$.  In particular, eq.~\eqref{eq:LQG_closed_reduction_step_1} holds since $J_t^\star(\calS)=\min_{u_t}[\mathbb{E}(\|x_{t+1}\|^2_{Q_t}+\|u_t\|^2_{R_t})+\min_{u_k \in \mathbb{R}^{m_k}, k\in \{t+1,\ldots,T\}}J_{t+1}(\calS, u_{t+1}, \ldots, u_T)]$; $J_{T+1}^\star(\calS)=0$ holds since the matrices $Q\at{T+1}$ and  $R_{T+1}$ are zero.  

We prove Lemma~\ref{lem:LQG_closed} for $t=T$.  From eq.~\eqref{eq:LQG_closed_reduction_step_1}, for $t=T$,
\beal
& J_T^\star(\calS)\\
&=\min_{u_T}\left[ \mathbb{E}(\|x_{T+1}\|^2_{Q_T}+\|u_T\|^2_{R_T})\right]\\
&=\min_{u_T}\left[ \mathbb{E}(\|A_Tx_T+B_Tu_T+w_T\|^2_{Q_T}+\|u_T\|^2_{R_T})\right],\label{eq:closed_aux_1}
\eeal
since $x_{T+1}=A_Tx_T+B_Tu_T+w_T$, per system Framework~\ref{frame:system}.  Therefore, from eq.~\eqref{eq:closed_aux_1},
\beal
& J_T^\star(\calS)\\
&=\min_{u_T}\left[\mathbb{E}(u_T\tran B_T\tran Q_T B_Tu_T+w_T\tran Q_Tw_T+\right.\\&\left. x_T\tran A_T\tran Q_TA_Tx_T+ 2x_T\tran A_T\tran Q_T B_Tu_T+2x_T\tran A_T\tran Q_T w_T+\right.\\&\left.2 u_T\tran B_T\tran Q_Tw_T+\|u_T\|^2_{R_T})\right]\\
&=\min_{u_T}\left[ \mathbb{E}(u_T\tran B_T\tran Q_T B_Tu_T+\|w_T\|_{Q_T}^2+ \right.\\&\left.x_T\tran A_T\tran Q_TA_Tx_T+ 2x_T\tran A_T\tran Q_T B_Tu_T+\|u_T\|^2_{R_T})\right],\label{eq:closed_aux_2}
\eeal
where the latter equality holds since $w_T$ has zero mean and $w_T$, $x_T$, and $u_T$ are independent.  From eq.~\eqref{eq:closed_aux_2}, completing the square between $u_T$ and $x_T$, and using the notation in eq.~\eqref{eq:control_riccati},
\beal
& J_T^\star(\calS)\\
&=\min_{u_T}\left[ \mathbb{E}(u_T\tran (B_T\tran Q_T B_T+R_T)u_T+\|w_T\|_{Q_T}^2+\right.\\&\left. x_T\tran A_T\tran Q_TA_Tx_T+ 2x_T\tran A_T\tran Q_T B_Tu_T\right]\\
&=\min_{u_T}\left[\mathbb{E}(\|u_T\|_{M_T}^2+\|w_T\|_{Q_T}^2+ x_T\tran A_T\tran Q_TA_Tx_T+\right.\\&\left. 2x_T\tran A_T\tran Q_T B_Tu_T\right]\\
&=\min_{u_T}\left[\mathbb{E}(\|u_T\|_{M_T}^2+\|w_T\|_{Q_T}^2+ x_T\tran A_T\tran  Q_TA_Tx_T-\right.\\&\left.2x_T\tran (-A_T\tran Q_T B_TM_T\inv) M_Tu_T\right]\\
&=\min_{u_T}\left[ \mathbb{E}(\|u_T\|_{M_T}^2+\|w_T\|_{Q_T}^2+ x_T\tran A_T\tran  Q_TA_Tx_T-\right.\\&\left.2x_T\tran K_T\tran M_Tu_T\right]\\
&=\min_{u_T}\left[ \mathbb{E}(\|u_T-K_Tx_T\|_{M_T}^2+\|w_T\|_{Q_T}^2+\right.\\&\left. x_T\tran (A_T\tran  Q_TA_T- K_T\tran M_T K_T)x_T\right]\\
&=\min_{u_T}\left(\frac{1}{2} \mathbb{E}(\|u_T-K_Tx_T\|_{M_T}^2+\|w_T\|_{Q_T}^2+\right.\\&\left. x_T\tran (A_T\tran  Q_TA_T- \Theta_T)x_T\right)\\
&=\min_{u_T}\left[ \mathbb{E}(\|u_T-K_Tx_T\|_{M_T}^2+\|w_T\|_{Q_T}^2+ \|x_T\|_{N_T}^2\right]\\
&=\min_{u_T} \mathbb{E}(\|u_T-K_Tx_T\|_{M_T}^2)+\trace{W_TQ_T}+ \\& \mathbb{E}( \|x_T\|_{N_T}^2),\label{eq:closed_aux_3}
\eeal
where the latter equality holds since $\mathbb{E}(\|w_T\|_{Q_T}^2)=\mathbb{E}\left[\trace{w_T\tran Q_Tw_T}\right]=\trace{\mathbb{E}(w_T\tran w_T)Q_T}=\trace{W_TQ_T}$.  From eq.~\eqref{eq:closed_aux_3}, we conclude that Lemma~\ref{lem:LQG_closed} holds for $t=T$, since for the first term in the last equality in~\eqref{eq:closed_aux_3},
\begin{align*}
\min_{u_T} \mathbb{E}(\|u_T-K_Tx_T\|_{M_T}^2)&=\mathbb{E}(\|K_T\hat{x}_{T,\calS}-K_Tx_T\|_{M_T}^2)\\
&=\trace{\Theta_T \Sigma\att{T}{T}(\calS)},
\end{align*}
since $\hat{x}_{T,\calS}$ is the minimum mean square estimator of $x_T$ given the measurements up to time $T$~\cite[Appendix~E]{bertsekas2005dynamic}.

We prove that if Lemma~\ref{lem:LQG_closed} holds for $t=l+1$, it also holds for $t=l$.  To this end, assume eq.~\eqref{eq:LQG_closed_reduction_step_1} holds for $t=l+1$.  Using the notation in eq.~\eqref{eq:control_riccati},
\beal
J_l^\star(\calS)&=\min_{u_l} \left[ \mathbb{E}(\|x_{l+1}\|^2_{Q_l}+\|u_l\|^2_{R_l})+ J_{l+1}^\star\right]\\
&=\min_{u_l} \left\{ \mathbb{E}(\|x_{l+1}\|^2_{Q_l}+\|u_l\|^2_{R_l})+ \mathbb{E}(\|x_{l+1}\|_{N_{l+1}}^2)+\right.\\
&\left.\sum_{k=l+1}^T\left[\trace{\Theta_k\Sigma\att{k}{k}(\calS)}+\trace{W_kS_k}\right]\right\}\\
&=\min_{u_l} \left\{ \mathbb{E}(\|x_{l+1}\|^2_{S_l}+\|u_l\|^2_{R_l})+\right.\\
&\left.\sum_{k=l+1}^T[\trace{\Theta_k\Sigma\att{k}{k}(\calS)}+\trace{W_kS_k}]\right\}\\
&=\sum_{k=l+1}^T[\trace{\Theta_k\Sigma\att{k}{k}(\calS)}+\trace{W_kS_k}]+\\
&\min_{u_l} \mathbb{E}(\|x_{l+1}\|^2_{S_l}+\|u_l\|^2_{R_l}).\label{eq:closed_aux_4}
\eeal

In eq.~\eqref{eq:closed_aux_4}, for the last term in the last equality,
\beal
&\min_{u_l} \mathbb{E}(\|x_{l+1}\|^2_{S_l}+\|u_l\|^2_{R_l})=\\
&\mathbb{E}(\|x_l\|_{N_l}^2)+\trace{\Theta_l\Sigma\att{l}{l}(\calS)}+\trace{W_lQ_l},\label{eq:closed_aux_5}
\eeal
and $u_l=K_l\hat{x}_{l,\calS}$, by following the same steps as for the proof of Lemma~\ref{lem:LQG_closed} for $t=T$.  Overall, if Lemma~\ref{lem:LQG_closed} holds for $t=l+1$, it also holds for $t=l$; hence, it also holds for $l=1$.
\end{proof}

\begin{proof}[Proof of Theorem~\ref{th:LQG_closed}]
We complete the proof in two steps: First, Eq.~\eqref{eq:opt_sensors} is implied from Lemma~\ref{lem:LQG_closed}'s eq.~\eqref{eq:lem:opt_sensors}, since for any sensor set $\calS\subseteq \calV$, both $\mathbb{E}(x_1\tran N_1 x_1)=\trace{\Sigma\att{1}{0}N_1}$ and $\sum_{t=1}^T\trace{W_tS_t}$ are independent of $\calS$.  Second,~\eqref{eq:opt_control} is implied from Lemma~\ref{lem:LQG_closed}'s eq.~\eqref{eq:lem:opt_control}.
\end{proof}

%\begin{mycorollary}
%\beq
%\min_{u_{1:T}}J_T=c+\frac{1}{2}\sum_{k=1}^T\left(\trace{A_t\tran S_t A_t\Sigma\att{t}{t}}+\trace{(Q_{t-1}-S_{t-1})\Sigma\att{t}{t}}\right),
%\eeq
%where $c=\frac{1}{2}\trace{N_1P\att{1}{0}}+\frac{1}{2}\sum_{k=1}^T\trace{W_tS_t}$.
%\end{mycorollary}
%\begin{proof}
%$\Theta_t=A_t\tran S_t A_t+Q_{t-1}-S_{t-1}$, since (i) $N_t =A_t\tran S_t A_t-\Theta_t$, and (ii) $-N_t=Q_{t-1}-S_{t-1}$, since $S_t=Q_t+N_{t+1}$.
%
%\end{proof}

\section*{Appendix B: Proof of Theorem~\ref{th:approx_bound}}

Due to separation theorem implied by Theorem~\ref{th:LQG_closed} in Appendix~A, it suffices to prove that the objective function in eq.~\eqref{eq:opt_sensors} is non-increasing.  To this end, we use the lemmata:

\begin{mylemma}[Proposition~8.5.5~\cite{bernstein2005matrix}]\label{lem:inverse}
For any positive definite matrices $M_1$ and $M_2$ such that $M_1\preceq M_2$, $M_2\inv\preceq M_1\inv$.

 
\end{mylemma}

\begin{mylemma}[Proposition 8.5.12~\cite{bernstein2005matrix}]\label{lem:traceAB_mon}
Consider symmetric matrices $A_1$ and $A_2$ such that $A_1\preceq A_2$, and a positive semi-definite matrix $B$; $\trace{A_1B}\leq \trace{A_2B}$.  
\end{mylemma}

\begin{mylemma}[Lemma~2.33~\cite{kumar1986stochastic}]
Consider $\Sigma\att{t+1}{t}$ and $\bar{\Sigma}\att{t+1}{t}$ to be the Kalman error covariances corresponding to initial conditions $\Sigma\att{1}{0}$ and $\bar{\Sigma}\att{1}{0}$. If $\Sigma\att{1}{0}\preceq\bar{\Sigma}\att{1}{0}$, $\Sigma\att{t+1}{t}\preceq\bar{\Sigma}\att{t+1}{t}$.  
\end{mylemma}

\begin{mycorollary}
Consider $\Sigma\att{t+1}{t}$ and $\bar{\Sigma}\att{t+1}{t}$ to be the Kalman error covariances corresponding to different initial conditions. If $\Sigma\att{t+1}{t}\preceq\bar{\Sigma}\att{t+1}{t}$, $\Sigma\att{t+2}{t+1}\preceq\bar{\Sigma}\att{t+2}{t+1}$.  
\end{mycorollary}


\begin{mylemma}\label{lem:monon_t_plus_1}
Consider $\Sigma\att{t}{t}$ and $\bar{\Sigma}\att{t}{t}$ to be the Kalman error covariances corresponding to different initial conditions. If $\Sigma\att{t}{t}\preceq\bar{\Sigma}\att{t}{t}$,  $\Sigma\att{t+1}{t}\preceq\bar{\Sigma}\att{t+1}{t}$.  
\end{mylemma}
\begin{proof}[Proof of Lemma~\ref{lem:monon_t_plus_1}]
From eq.~\eqref{eq:covariance_riccati}, $\Sigma\att{t+1}{t} = A_{t} \Sigma\att{t}{t} A_{t}\tran + W_{t} \preceq A_{t} \bar{\Sigma}\att{t}{t} A_{t}\tran+W_{t}= \bar{\Sigma}\att{t+1}{t} $, since if $\Sigma\att{t}{t}\preceq\bar{\Sigma}\att{t}{t}$, $A_{t} \Sigma\att{t}{t} A_{t}\tran \preceq A_{t} \bar{\Sigma}\att{t}{t} A_{t}\tran$.
\end{proof}

\begin{mylemma}\label{lem:t_plus_1}
Consider $\Sigma\att{t}{t-1}$ and $\bar{\Sigma}\att{t}{t-1}$ to be the Kalman error covariances corresponding to different initial conditions. If $\Sigma\att{t}{t-1}\preceq\bar{\Sigma}\att{t}{t-1}$,  $\Sigma\att{t}{t}\preceq\bar{\Sigma}\att{t}{t}$.  
\end{mylemma}
\begin{proof}[Proof of Lemma~\ref{lem:t_plus_1}]
From eq.~\eqref{eq:covariance_riccati}, $\Sigma\att{t}{t} =(\Sigma\att{t}{t-1}\inv+C_t\tran V_t\inv C_t)\inv  \preceq (\bar{\Sigma}\att{t}{t-1}\inv+C_t\tran V_t\inv C_t)\inv= \bar{\Sigma}\att{t}{t} $, since Lemma~\ref{lem:inverse} and the condition $\Sigma\att{t}{t-1}\preceq\bar{\Sigma}\att{t}{t-1}$ implies $\Sigma\att{t}{t-1}\inv+C_t\tran V_t\inv C_t\succeq \bar{\Sigma}\att{t}{t-1}\inv+C_t\tran V_t\inv C_t$, which in turn implies $(\Sigma\att{t}{t-1}\inv+C_t\tran V_t\inv C_t)\inv  \preceq (\bar{\Sigma}\att{t}{t-1}\inv+C_t\tran V_t\inv C_t)\inv$.
\end{proof}

\begin{mylemma}\label{lem:monon_t}
Consider $\Sigma\att{t}{t}$ and $\bar{\Sigma}\att{t}{t}$ to be the conditional covariances corresponding to different initial conditions. If $\Sigma\att{t}{t}\preceq\bar{\Sigma}\att{t}{t}$, $\Sigma\att{t+1}{t+1}\preceq\bar{\Sigma}\att{t+1}{t+1}$.  
\end{mylemma}
\begin{proof}[Proof of Lemma~\ref{lem:monon_t}]
If $\Sigma\att{t}{t}\preceq\bar{\Sigma}\att{t}{t}$, from Lemma~\ref{lem:monon_t_plus_1}, $\Sigma\att{t+1}{t}\preceq\bar{\Sigma}\att{t+1}{t}$, which due Lemma~\ref{lem:t_plus_1} implies  $\Sigma\att{t+1}{t+1}\preceq\bar{\Sigma}\att{t+1}{t+1}$.
\end{proof}


\begin{mylemma}\label{prop:one-step_monotonicity}
For any sensor sets $\calS_1\subseteq \calS_2 \subseteq \calV$,  $\Sigma\att{1}{1}(\calS_1)\succeq \Sigma\att{1}{1}(\calS_2)$.  
\end{mylemma}
\begin{proof}
Let $\calD=\calS_2\setminus \calS_1$, and observe 
\begin{align*}
& C_1(\calS_2)\tran V_t(\calS_2)\inv C_t(\calS_2)=\\ & C_1(\calS_1)\tran V_t(\calS_1)\inv C_t(\calS_1)+C_1(\calD)\tran V_t(\calD)\inv C_t(\calD)\succeq\\
& C_1(\calS_1)\tran V_t(\calS_1)\inv C_t(\calS_1);
\end{align*}
therefore, eq.~\eqref{eq:covariance_riccati} and Lemma~\ref{lem:inverse} imply 
\begin{align*}
&\Sigma\att{1}{1}(\calS_2) =\\
&[\Sigma\att{1}{0}\inv+C_1(\calS_2)\tran V_t(\calS_2)\inv C_t(\calS_2)]\inv\preceq\\
& [\Sigma\att{1}{0}\inv+C_1(\calS_1)\tran V_t(\calS_1)\inv C_t(\calS_1)]\inv=\\
&\Sigma\att{1}{1}(\calS_1).
\end{align*} 
%Since $\Theta_1$ is symmetric, Lemma~\ref{prop:one-step_monotonicity} is implied by Lemma~\ref{lem:traceAB_mon}.
\end{proof}

\begin{myproposition}\label{prop:monotonicity}
For any sensor set $\calS\subseteq \calV$, consider the set function $\sum_{t=1}^{T}\trace{\Theta_t \Sigma\att{t}{t}(\calS)}$; for any sensor sets $\calS_1\subseteq \calS_2 \subseteq \calV$,  $\sum_{t=1}^{T}\trace{\Theta_t \Sigma\att{t}{t}(\calS_1)}\geq \sum_{t=1}^{T}\trace{\Theta_t \Sigma\att{t}{t}(\calS_2)}$.  
\end{myproposition}
\begin{proof}
Lemma~\ref{prop:one-step_monotonicity} and Lemma~\ref{lem:monon_t} imply $\Sigma\att{t}{t}(\calS_1) \succeq \Sigma\att{t}{t}(\calS_2)$; and for any time $t\in \until{T}$, Lemma~\ref{lem:traceAB_mon} implies $\trace{\Theta_t \Sigma\att{t}{t}(\calS_1)}\geq \trace{\Theta_t \Sigma\att{t}{t}(\calS_2)}$, since $\Theta_t$ is symmetric.
%Assume that an element $v$ is added in $\calS_i$, for some $1\leq i\leq t$, and let $\calS_i'=\calS_i \cup \{v\}$. From~\eqref{eq:covariance_riccati}, 
%\begin{itemize}
%\item for $t\leq i-1$, $\trace{\Theta_t \Sigma\att{t}{t}}$ remains unaffected by this change, since $\calS_t$ remains the same; 
%\item for $t=i$, $\trace{\Theta_t \Sigma\att{t}{t}'}\leq \trace{\Theta_1 \Sigma\att{t}{t}}$, since (i)~$\Sigma\att{t}{t}'\preceq \Sigma\att{t}{t}$ due to~\eqref{eq:covUpdate}, because $\calS_t'=\calS_t\cup \{v\}\supseteq \calS_t$ and $\Sigma\att{t}{t-1}=\Sigma\att{t}{t-1}'$, and (ii)~Lemma~\ref{lem:traceAB_mon}.
%\end{itemize}
\end{proof}

\begin{proof}[Proof of part~(1) of Theorem~\ref{th:approx_bound} (Algorithm~\ref{alg:greedy}'s approximation quality)] The proof of Theorem~\ref{th:approx_bound}'s approximation bound in ineq.~\eqref{ineq:approx_bound} is implied by Proposition~\ref{prop:monotonicity},~\cite[Theorem~2]{wang2016approximation}, and~\cite[Theorem~1]{chamon2016near}.
\end{proof}

\begin{proof}[Proof of part~(2) of Theorem~\ref{th:approx_bound} (Algorithm~\ref{alg:greedy}'s running time)]
We compute Algorithm~\ref{alg:greedy}'s running time by adding the running time of lines 1--5, 6--9, and 10--23:

\textit{a)} Lines 1--5 need $O(n^{2.4})$ time, using the Coppersmith algorithm for both matrix inversion and multiplication~\cite{coppersmith1990matrix}.

\textit{b)} Lines 6--9 need $O(n^{2.4})$ time, using the Coppersmith algorithm for both matrix inversion and multiplication~\cite{coppersmith1990matrix}.

\textit{c)} Lines 10--23 need $O(k|\calV|Tn^{2.4}+k|\calV|+k|\calV|n^{2.4}+k|\calV|\log(|\calV|))$ time, since: (i)~the lines 12--20 are repeated at most $k$ times, due to the while loop between in line~12, and each repetition of lines 12--20 needs $O(|\calV|Tn^{2.4})$ time, using the Coppersmith-Winograd algorithm for both matrix inversion and multiplication~\cite{coppersmith1990matrix}; (ii)~the lines 21--22 are repeated at most $k$ times, due to the while loop in line~12, and each repetition of lines 21--22 needs $O(|\calV|n^{2.4}+|\calV|\log(|\calV|)$ time, since line 21 asks (ii.a)~for at most $|\calV|$ evaluations of $\sum_{t=1}^T\text{tr}[\Theta_t\Sigma\att{t}{t}(\cdot)]$, which take $O(|\calV|n^{2.4})$, using the Coppersmith-Winograd algorithm for both matrix multiplication~\cite{coppersmith1990matrix}; and (ii.b)~for the minimum among at most~$|\calV|$ values of $\sum_{t=1}^T\text{tr}[\Theta_t\Sigma\att{t}{t}(\cdot)]$, which takes $\log[|\calV|\log(|\calV|)]$ time, using, e.g., the merge sort algorithm.

In sum, Algorithm~\ref{alg:greedy}'s running time is $O(n^{2.4}+n^{2.4}+k|\calV|Tn^{2.4}+k|\calV|+k|\calV|n^{2.4}+k|\calV|\log(|\calV|)=O(k|\calV|Tn^{2.4})$.
\end{proof}
%\begin{lemma}
%Consider matrices $A$ and $B$ such that $A$ and $A+B$ are invertible.
%\begin{align}
%(A+B)^{-1}&=A^{-1}-A^{-1}B(A+B)^{-1}\label{eq:aux_lemma_1}\\
%&=A^{-1}-(A+B)^{-1}BA^{-1} \label{eq:aux_lemma_2}
%\end{align}
%\end{lemma}
%\begin{proof}
%Let's prove~\eqref{eq:aux_lemma_1}. Multiplying its right hand side with $A+B$,
%\begin{align}
%A^{-1}(A+B)-A^{-1}B&=I+A^{-1}B-A^{-1}B\\
%&=I.
%\end{align}
%\end{proof}

%
%
%\begin{mylemma}\label{lem:positive_def_Theta}
%If $B_t$ is full row rank, and $A_t$ is invertible, $\Theta_t\succ 0$.
%\end{mylemma}
%\begin{proof}
%Let vector $z$ such that $\Theta_tz=0$. In addition, let an invertible matrix $M_1$ such that $M_t=M_1\tran M_1$; such matrix exists since $M_t$ is positive definite (Theorem 3.7,~\cite{chi-TsongChen}). Then:
%\beal
%K_t\tran M_t K_t z &=0 \Rightarrow\\
%M_1 K_t z &=0 \Rightarrow\\
%K_t z &=0 \Rightarrow\\
%-M_t\inv B_t\tran S_t A_t z &=0 \Rightarrow\\
%B_t\tran S_t A_t z &=0\Rightarrow\\
%S_t A_t z &=0\Rightarrow\\
%A_t z &=0\Rightarrow\\
%z &=0.\\
%\eeal
%\end{proof}
%
%\begin{mytheorem}[Supermodularity ratio]
%\end{mytheorem}
%\begin{proof}
%Let $f(\calS)=\trace{\Theta_t \Sigma\att{t}{t}(\calS)}$.
%
%Add a new element $\{v\}$ in $\calS$. Then, $$\Sigma\att{t}{t}(\calS\cup \{v\})=\left(\Sigma\att{t}{t-1}\inv(\calS \cup \{v\})+\sum_{i \in \calS \cup \{v\}} c_i\tran c_i\right)\inv.$$
%Let $\Omega_{\calS}=\Sigma\att{t}{t-1}\inv(\calS)+\sum_{i \in \calS}\inv c_i\tran c_i$, and $\Omega_{\calS\cup \{v\}}=\Sigma\att{t}{t-1}\inv(\calS\cup \{v\})+\sum_{i \in \calS}\inv c_i\tran c_i$.
% 
%\beal
%f(\calS\cup \{v\})&=\trace{\Theta_t\Omega_{\calS\cup \{v\}}\inv}-\trace{\Theta_t\frac{\Omega_{\calS\cup \{v\}}\inv c_i\tran c_i \Omega_{\calS\cup \{v\}}\inv}{1+c_i\tran \Omega_{\calS\cup \{v\}}\inv c_i}}.
%\eeal
%
%Towards computing a lower bound to the submodularity ratio $\gamma_f$, let $\calS \subseteq \calS'$. For the numerator, 
%\beal
%& f(\calS)-f(\calS\cup \{v\})=
%\\
%& \trace{\Theta_t\Omega_{\calS}\inv}-\trace{\Theta_t\Omega_{\calS\cup \{v\}}\inv}+\trace{\Theta_t\frac{\Omega_{\calS\cup \{v\}}\inv c_i\tran c_i \Omega_{\calS\cup \{v\}}\inv}{1+c_i\tran \Omega_{\calS\cup \{v\}}\inv c_i}}\\
%&\geq \trace{\Theta_t\frac{\Omega_{\calS\cup \{v\}}\inv c_i\tran c_i \Omega_{\calS\cup \{v\}}\inv}{1+c_i\tran \Omega_{\calS\cup \{v\}}\inv c_i}}\\
%&\geq \lambda_\min(\Theta_t)\frac{ c_i\tran \Omega_{\calS\cup \{v\}}^{-2}c_i}{1+c_i\tran \Omega_{\calS\cup \{v\}}\inv c_i}\\
%&\geq \lambda_\min(\Theta_t)\frac{ c_i\tran \Omega_{\mathcal{V}}^{-2}c_i}{1+c_i\tran \Omega_{\emptyset}\inv c_i}\\
%&\text{\VT{or better the following,}} \\ 
%&\text{\VT{since for $B$ non full row rank, $\lambda_\min(\Theta_t)=0$:}}\\
%&= \frac{ c_i\tran \Omega_{\calS\cup \{v\}}\inv\Theta_t\Omega_{\calS\cup \{v\}}\inv c_i}{1+c_i\tran \Omega_{\calS\cup \{v\}}\inv c_i},
%\eeal
%because $\trace{\Theta_t\Omega_{\calS}\inv}\geq \trace{\Theta_t\Omega_{\calS\cup \{v\}}\inv}$ since (i)~$\Omega_{\calS\cup \{v\}}\inv \preceq\Omega_{\calS}\inv$, since $\Omega_{\calS\cup \{v\}} \succeq\Omega_{\calS}$, since  $\Sigma\att{t}{t-1}\inv(\calS\cup \{v\})\succeq \Sigma\att{t}{t-1}\inv(\calS)$, since $\Sigma\att{t}{t-1}(\calS\cup \{v\})\preceq \Sigma\att{t}{t-1}(\calS)$, and (ii)~Lemma~\ref{lem:traceAB_mon}.
%
%For the denominator, first observe
%\beal
%\Sigma\att{t}{t}(\calS'\cup \{v\})&=\left(\Omega_{\calS'\cup \{v\}} + c_v\tran c_v\right)\inv \preceq \left(\Omega_{\calS'} + c_v\tran c_v\right)\inv\\
%\Sigma\att{t}{t}(\calS')&=\Omega_{\calS'}\inv \succeq \Omega_{\calS'\cup\{v\}}\inv ,
%\eeal
%since $\Omega_{\calS\cup \{v\}}\inv \preceq\Omega_{\calS}\inv$.
%\beal
%& f(\calS')-f(\calS'\cup \{v\})=
%\\
%& \trace{\Theta_t\Omega_{\calS'}\inv}-\trace{\Theta_t\Omega_{\calS'\cup \{v\}}\inv}+\trace{\Theta_t\frac{\Omega_{\calS'\cup \{v\}}\inv c_i\tran c_i \Omega_{\calS'\cup \{v\}}\inv}{1+c_i\tran \Omega_{\calS'\cup \{v\}}\inv c_i}}\\
%&\leq \trace{\Theta_t\Omega_{\calS'}\inv}+\trace{\Theta_t\frac{\Omega_{\calS'\cup \{v\}}\inv c_i\tran c_i \Omega_{\calS'\cup \{v\}}\inv}{1+c_i\tran \Omega_{\calS'\cup \{v\}}\inv c_i}}\\
%&\leq \lambda_\max(\Theta_t) \trace{\Omega_\emptyset\inv}+\lambda_\max(\Theta_t)\frac{ c_i\tran \Omega_{\emptyset}^{-2}c_i}{1+c_i\tran \Omega_{\mathcal{V}}\inv c_i}.
%\eeal
%\end{proof}
%
%\begin{mylemma}[Fact 8.14.10~\cite{bernstein2005matrix}]\label{lem:lower_bound_trace_sum_eigen}
%Consider a non-negative integer $n$, and two positive semi-definite matrices $A$ and $B$, both of size $n \times n$. Let $\lambda_1(A), \lambda_2(A), \ldots, \lambda_n(A)$ denote the eigenvalues of $A$ such that $\lambda_1(A)\geq \lambda_2(A)\geq \ldots\geq \lambda_n(A)$, and similarly for the matrix $B$.
%\beq
%\sum_{k=1}^{n}\lambda_i(A)\lambda_{n-k+1}(B)\leq \trace{AB}.
%\eeq
%\end{mylemma}
%
%\begin{mytheorem}[Suff. conditions for non-vanishing sub. ratio]
%
%\mbox{ }
%
%\begin{itemize}
%
%\item Consider that at time step $t$, $\Theta_t$ has rank $\theta_t$. If, any sensor matrix $C_{i,t}$ has rank at least $n-\theta_t+1$, the submodularity ratio is non-vanishing; in particular, the numerator of $\gamma_t$ is lower bounded by
%\end{itemize}
%\beal
%&\lambda_{\theta_t}(\Theta_t) \times\\
%&\min_{i,\calS}\lambda_{n-\theta_t+1}(\Omega_{\calS\cup \{i\}}\inv C_{i,t}\tran (I+C_{i,t}\tran \Omega_{\calS\cup \{i\}}\inv C_{i,t})\inv C_{i,t}\Omega_{\calS\cup \{i\}}\inv).
%\eeal
%
%\begin{itemize}
%\item Consider that at time step $t$, $B_t$ has full row rank, and $A_t$ is invertible. The submodularity ration is non-vanishing; in particular, the numerator of $\gamma_t$ is lower bounded by 
%\end{itemize}
%\beal
%& \lambda_{\min}(\Theta_t)\times\\
%&\min_{i,\calS}\trace{\Omega_{\calS\cup \{i\}}\inv C_{i,t}\tran (I+C_{i,t}\tran \Omega_{\calS\cup \{i\}}\inv C_{i,t})\inv C_{i,t}\Omega_{\calS\cup \{i\}}\inv}.
%\eeal
%
%
%\begin{itemize}
%\item {\color{red} If we consider the LQR problem, where in the cost function we add the term $\sum_{t=1}^Tx_t\tran L_t u_t$, where $L_t$ invertible, then $\Theta_t^{\text{LQR}}$ becomes $\Theta_t^{\text{LQG}}+L_tM_tL_t\tran \succ 0$. That is, the numerator of the submodularity ratio is bounded by}
%\end{itemize}
%\beal
%& \lambda_{\min}(\Theta_t^{\text{LQR}})\times\\
%&\min_{i,\calS}\trace{\Omega_{\calS\cup \{i\}}\inv C_{i,t}\tran (I+C_{i,t}\tran \Omega_{\calS\cup \{i\}}\inv C_{i,t})\inv C_{i,t}\Omega_{\calS\cup \{i\}}\inv} \\
%&\geq \lambda_{\min}(\Theta_t^{\text{LQR}})\times\\
%&\min_i\trace{\Omega_{\mathcal{V}}\inv C_{i,t}\tran (I+C_{i,t}\tran \Omega_{\emptyset}\inv C_{i,t})\inv C_{i,t}\Omega_{\mathcal{V}}\inv}.
%\eeal
%
%\end{mytheorem}
%\begin{proof}
%\begin{enumerate}
%\item It follows from Lemma~\ref{lem:lower_bound_trace_sum_eigen}, and the fact that if $C_{i,t}$ has rank $n-\theta_t+1$ then $$\lambda_{n-\theta_t+1}(\Omega_{\calS}\inv C_{i,t}\tran (I+C_{i,t}\tran \Omega_{\calS}\inv C_{i,t})\inv C_{i,t}\Omega_{\calS})>0.$$
%\item If $B_t$ has full row rank, and $A_t$ is invertible, $\Theta_t$ is invertible, that is, $\lambda_{\min}(\Theta_t)>0$.
%\end{enumerate}
%
%\end{proof}

\section*{Appendix C: Proof of Theorem~\ref{th:submod_ratio}}


For the proof of Theorem~\ref{th:submod_ratio}, we use Lemmata~\ref{lem:trace_low_bound_lambda_min} and~\ref{lem:woodbury}.

\begin{mylemma}[Proposition~8.4.13 in~\cite{bernstein2005matrix}]\label{lem:trace_low_bound_lambda_min}
Consider a symmetric matrix $A$, and a positive semi-definite matrix $B$ of appropriate dimension.
\begin{equation*}
\lambda_\min(A)\trace{B}\leq \trace{AB}\leq \lambda_\max(A)\trace{B}.
\end{equation*}
\end{mylemma}

\begin{mylemma}[Woodbury identity (\hspace{-.05mm}\cite{bernstein2005matrix}, Corollary 2.8.8)]\label{lem:woodbury}
Consider matrices $A$, $C$, $U$ and $V$ such that $A$, $C$, and $A+UCV$ are invertible.
\begin{equation*}
(A+UCV)\inv=A\inv-A\inv U(C\inv+VA\inv U)\inv VA\inv.
\end{equation*}
\end{mylemma}
We complete the proof of Theorem~\ref{th:submod_ratio} in two steps: first, we derive a non-zero low bound for the supermodularity ratio $\gamma_g$ for the case where only $\sum_{t=1}^{T}\Theta_t\succ 0$; second, we prove the supermodularity ratio bound in ineq.~\eqref{ineq:sub_ratio_bound}. To this end, we use the following notation. 

\begin{mynotation}
Let 
\begin{itemize}
\item $c=\mathbb{E}(x_1\tran N_1 x_1)+\sum_{t=1}^T\trace{W_tS_t}$;
\item for any sensor set $\calS \subseteq \calV$, and for any time $t \in \until{T}$, $f_t(\calS)=\trace{\Theta_t \Sigma\att{t}{t}(\calS)}$.
\end{itemize}  
Due to Lemma~\ref{lem:LQG_closed}, for any sensor set $\calS \subseteq \calV$,  $$g(\calS)=c+\sum_{t=1}^T f_t(\calS).$$
\end{mynotation}

\begin{proof}[Proof of Theorem~\ref{th:submod_ratio} for the case where only $\sum_{t=1}^{T}\Theta_t\succ 0$]
We complete the proof by first deriving a worst-case lower bound for the numerator in the supermodularity ratio Definition~\ref{def:super_ratio}, and then, by deriving a worst-case upper bound for the denominator in the supermodularity ratio Definition~\ref{def:super_ratio}.

\textit{a)~Worst-case lower bound for the numerator in the supermodularity ratio Definition~\ref{def:super_ratio}:} The numerator of the submodularity ratio $\gamma_g$ is of the form
\begin{equation}\label{eq:ratio_aux_1}
\sum_{t=1}^{T}[f_t(\calS)-f_t(\calS\cup \{v\})],
\end{equation}
for some sensor set $\calS\subseteq \calV$, and sensor $v \in \calV$; to lower bound the sum in~\eqref{eq:ratio_aux_1}, for any time $t \in \until{T}$, we bound $f_t(\calS)-f_t(\calS\cup \{v\})$.
To this end, from~eq.~\eqref{eq:covariance_riccati}, observe
\begin{equation*}
\Sigma\att{t}{t}(\calS\cup \{v\})=[\Sigma\att{t}{t-1}\inv(\calS \cup \{v\})+\sum_{i \in \calS \cup \{v\}} \bar{C}_{i,t}\tran \bar{C}_{i,t}]\inv.
\end{equation*}
Consider $\Omega_t=\Sigma\att{t}{t-1}\inv(\calS)+\sum_{i \in \calS}^T \bar{C}_{i,t}\tran \bar{C}_{i,t}$, and $\bar{\Omega}_{t}=\Sigma\att{t}{t-1}\inv(\calS\cup \{v\})+\sum_{i \in \calS}^T \bar{C}_{i,t}\tran \bar{C}_{i,t}$; using the Woodbury identity in Lemma~\ref{lem:woodbury}, 
\begin{align*}
f_t(\calS\cup \{v\})&=\trace{\Theta_t\bar{\Omega}_{t}\inv}-\\
&\hspace{0.4em}\trace{\Theta_t\bar{\Omega}_{t}\inv \bar{C}_{v,t}\tran (I+\bar{C}_{v,t} \bar{\Omega}_{t}\inv \bar{C}_{v,t}\tran)\inv \bar{C}_{v,t} \bar{\Omega}_{t}\inv}.
\end{align*}
Therefore, for any time $t \in \until{T}$,
\begin{align}
& f_t(\calS)-f_t(\calS\cup \{v\})=
\nonumber\\
&\trace{\Theta_t\Omega_{t}\inv}-\trace{\Theta_t\bar{\Omega}_{t}\inv}+\nonumber\\
&\trace{\Theta_t\bar{\Omega}_{t}\inv \bar{C}_{v,t}\tran (I+\bar{C}_{v,t} \bar{\Omega}_{t}\inv \bar{C}_{v,t}\tran)\inv \bar{C}_{v,t} \bar{\Omega}_{t}\inv}\geq\nonumber\\
& \trace{\Theta_t\bar{\Omega}_{t}\inv \bar{C}_{v,t}\tran (I+\bar{C}_{v,t} \bar{\Omega}_{t}\inv \bar{C}_{v,t}\tran)\inv \bar{C}_{v,t} \bar{\Omega}_{t}\inv},\label{ineq:super_ratio_aux_1}
\end{align}
where ineq.~\eqref{ineq:super_ratio_aux_1} holds because $\trace{\Theta_t\Omega_{t}\inv}\geq \trace{\Theta_t\bar{\Omega}_{t}\inv}$, which is implied by Lemma~\ref{lem:traceAB_mon} in Appendix~B, since $\Theta_t$ is a symmetric matrix, and $\Omega_{t}\inv\succeq \bar{\Omega}_{t}\inv$; in particular, $\Omega_{t}\inv\succeq \bar{\Omega}_{t}\inv$ is implied by Lemma~\ref{lem:inverse}, since $\Omega_{t}\preceq \bar{\Omega}_{t} $; in more detail, $\Omega_{t}\preceq \bar{\Omega}_{t} $ because $\Sigma\att{t}{t-1}(\calS)\inv\preceq\Sigma\att{t}{t-1}(\calS\cup\{u\})\inv$, which is implied by $ \Sigma\att{t}{t-1}(\calS)\succeq \Sigma\att{t}{t-1}(\calS\cup \{v\})$, which holds from Lemma~\ref{lem:monon_t_plus_1} and the fact that $\Sigma\att{1}{1}(\calS)\succeq\Sigma\att{1}{1}(\calS\cup\{u\})$, which is implied by Lemma~\ref{prop:one-step_monotonicity}.  From the ineq.~\eqref{ineq:super_ratio_aux_1},
\begin{align}
& f_t(\calS)-f_t(\calS\cup \{v\})\geq\nonumber \\
&\trace{\bar{C}_{v,t} \bar{\Omega}_{t}\inv \Theta_t\bar{\Omega}_{t}\inv \bar{C}_{v,t}\tran (I+\bar{C}_{v,t} \bar{\Omega}_{t}\inv \bar{C}_{v,t}\tran)\inv }\geq \nonumber\\
&\lambda_\min((I+\bar{C}_{v,t} \bar{\Omega}_{t}\inv \bar{C}_{v,t}\tran)\inv)\trace{\bar{C}_{v,t} \bar{\Omega}_{t}\inv \Theta_t\bar{\Omega}_{t}\inv \bar{C}_{v,t}\tran },\label{ineq:super_ratio_aux_2}
\end{align}
where ineq.~\eqref{ineq:super_ratio_aux_2} holds due to Lemma~\ref{lem:trace_low_bound_lambda_min}.  From ineq.~\eqref{ineq:super_ratio_aux_2},
\begin{align}
& f_t(\calS)-f_t(\calS\cup \{v\})\geq\nonumber \\
&= \lambda_\max\inv(I+\bar{C}_{v,t} \bar{\Omega}_{t}\inv \bar{C}_{v,t}\tran)\trace{\bar{C}_{v,t} \bar{\Omega}_{t}\inv \Theta_t\bar{\Omega}_{t}\inv \bar{C}_{v,t}\tran }\nonumber\\
&\geq \lambda_\max\inv(I+\bar{C}_{v,t} \Sigma\att{t}{t}(\emptyset) \bar{C}_{v,t}\tran)\trace{\bar{C}_{v,t} \bar{\Omega}_{t}\inv \Theta_t\bar{\Omega}_{t}\inv \bar{C}_{v,t}\tran }\nonumber\\
&= \lambda_\max\inv(I+\bar{C}_{v,t} \Sigma\att{t}{t}(\emptyset) \bar{C}_{v,t}\tran)\trace{\Theta_t \bar{\Omega}_{t}\inv \bar{C}_{v,t}\tran \bar{C}_{v,t}\bar{\Omega}_{t}\inv},\label{ineq:super_ratio_aux_3}
\end{align}
where we used $\Sigma\att{t}{t}(\emptyset)\succeq \bar{\Omega}_{t}\inv$, which holds because of the following: (i)~$\bar{\Omega}_{t}\succeq \Sigma\inv\att{t}{t-1}(\calS\cup \{v\})$, and as a result, $\bar{\Omega}_{t}\inv \preceq \Sigma\att{t}{t-1}(\calS\cup \{v\})$; (ii)~$\Sigma\att{t}{t-1}(\calS\cup \{v\})\preceq \Sigma\att{t}{t-1}(\emptyset)$, due to Lemma~\ref{lem:monon_t_plus_1} and the fact that $\Sigma\att{1}{1}(\calS\cup \{v\})\preceq \Sigma\att{1}{1}(\emptyset)$, which holds due to Lemma~\ref{prop:one-step_monotonicity}; and (iii)~$\Sigma\att{t}{t-1}(\emptyset)=\Sigma\att{t}{t}(\emptyset)$. 

Consider a time $t' \in \until{T}$ such that for any time $t \in \{1,2,\ldots,T\}$, $\bar{\Omega}_{t'}\inv \bar{C}_{v,t'}\tran \bar{C}_{v,t'}\bar{\Omega}_{t'}\inv  \preceq  \bar{\Omega}_{t}\inv \bar{C}_{v,t}\tran \bar{C}_{v,t} \bar{\Omega}_{t}\inv $, and let $\Phi$ to be the matrix $\bar{\Omega}_{t'}\inv \bar{C}_{v,t'}\tran \bar{C}_{v,t'} \bar{\Omega}_{t'}\inv $; similarly, let $l$ to be the $\min_{t\in\until{T},u \in \calV}\lambda_\max\inv(I+\bar{C}_{v,t} \Sigma\att{t}{t}(\emptyset) \bar{C}_{v,t}\tran)$. 
Summing ineq.~\eqref{ineq:super_ratio_aux_3} across all times $t \in \until{T}$, and using Lemmata~\ref{lem:traceAB_mon} and~\ref{lem:trace_low_bound_lambda_min},
\begin{align*}
 g(\calS)-g(\calS\cup\{v\})&\geq  l\sum_{t=1}^T \trace{\Theta_t\bar{\Omega}_{t}\inv \bar{C}_{v,t}\tran \bar{C}_{v,t} \bar{\Omega}_{t}\inv }\\
& \geq l\sum_{t=1}^T \trace{\Theta_t \Phi}\\
& =l\trace{\Phi \sum_{t=1}^T \Theta_t }\\
& \geq l \lambda_\min\left(\sum_{t=1}^T \Theta_t \right)\trace{\Phi}\\
&>0,
\end{align*}
which is non-zero because $\sum_{t=1}^T \Theta_t\succ 0$ and $\Phi$ is a non-zero positive semi-definite matrix. 

Finally, we lower bound $\trace{\Phi}$, using Lemma~\ref{lem:trace_low_bound_lambda_min}:
\begin{align}
\trace{\Phi}&=\trace{\bar{\Omega}_{t'}\inv \bar{C}_{v,t'}\tran \bar{C}_{v,t'} \bar{\Omega}_{t'}\inv }\nonumber\\
&=\trace{ \bar{\Omega}_{t'}^{-2} \bar{C}_{v,t'}\tran\bar{C}_{v,t'}}\nonumber\\
&\geq \lambda_\min(\bar{\Omega}_{t'}^{-2}) \trace{\bar{C}_{v,t'}\tran\bar{C}_{v,t'}}\nonumber\\
&= \lambda_\min^2(\bar{\Omega}_{t'}^{-1}) \trace{\bar{C}_{v,t'}\tran\bar{C}_{v,t'}}\nonumber\\
&\geq \lambda_\min^2(\Sigma\att{t'}{t'}(\calV)) \trace{\bar{C}_{v,t'}\tran\bar{C}_{v,t'}},\label{ineq:super_ratio_aux_10}
\end{align}
where ineq.~\eqref{ineq:super_ratio_aux_10} holds because $\bar{\Omega}_{t'}^{-1}\succeq \Sigma\att{t'}{t'}(\calS\cup \{v\})\succeq \Sigma\att{t'}{t'}(\calV)$; in particular, $\bar{\Omega}_{t'}^{-1}\succeq \Sigma\att{t'}{t'}(\calS\cup \{v\})$ holds because $\bar{\Omega}_{t'}\preceq \bar{\Omega}_{t'}+\bar{C}_{v,t}\tran\bar{C}_{v,t}\tran=\Sigma\inv\att{t'}{t'}(\calS\cup\{v\})$.  In addition, $\Sigma\att{t'}{t'}(\calS\cup \{v\})\succeq \Sigma\att{t'}{t'}(\calV)$ is implied from Lemma~\ref{lem:monon_t}, because $\Sigma\att{1}{1}(\calS\cup \{v\})\succeq \Sigma\att{1}{1}(\calV)$, due to Lemma~\ref{prop:one-step_monotonicity}.

\textit{b)~Worst-case upper bound for the denominator in the supermodularity ratio Definition~\ref{def:super_ratio}:} The denominator of the submodularity ratio $\gamma_g$ is of the form
\begin{equation*}
\sum_{t=1}^{T}[f_t(\calS')-f_t(\calS'\cup \{v\})],
\end{equation*}
for some sensor set $\calS'\subseteq \calV$, and sensor $v \in \calV$;  to upper bound it, observe
\begin{equation*}
\Sigma\att{t}{t}(\calS'\cup \{v\})=[\Sigma\att{t}{t-1}\inv(\calS' \cup \{v\})+\sum_{i \in \calS' \cup \{v\}} \bar{C}_{i,t}\tran \bar{C}_{i,t}]\inv,
\end{equation*}
and let $H_t=\Sigma\att{t}{t-1}\inv(\calS')+\sum_{i \in \calS'}^T\bar{C}_{i,t}\tran \bar{C}_{i,t}$, and $\bar{H}_{t}=\Sigma\att{t}{t-1}\inv(\calS'\cup \{v\})+\sum_{i \in \calS'}^T \bar{C}_{i,t}\tran \bar{C}_{i,t}$; using the Woodbury identity in Lemma~\ref{lem:woodbury},
\begin{align*}
f_t(\calS'\cup \{v\})&=\trace{\Theta_t\bar{H}_{t}\inv}-\\
&\hspace{0.4em}\trace{\Theta_t\bar{H}_{t}\inv \bar{C}_{v,t}\tran (I+\bar{C}_{v,t} \bar{H}_{t}\inv \bar{C}_{v,t}\tran)\inv \bar{C}_{v,t} \bar{H}_{t}\inv}.
\end{align*}
Therefore, 
\begin{align}
&\sum_{t=1}^T [f_t(\calS')-f_t(\calS'\cup \{v\})]=
\nonumber\\
&\sum_{t=1}^T [\trace{\Theta_t H_{t}\inv}-\trace{\Theta_t\bar{H}_{t}\inv}+\nonumber\\
&\trace{\Theta_t\bar{H}_{t}\inv \bar{C}_{v,t}\tran (I+\bar{C}_{v,t} \bar{H}_{t}\inv \bar{C}_{v,t}\tran)\inv \bar{C}_{v,t} \bar{H}_{t}\inv}]\leq\nonumber\\
&\sum_{t=1}^T [\trace{\Theta_t H_{t}\inv}+ \nonumber\\
&\trace{\Theta_t\bar{H}_{t}\inv \bar{C}_{v,t}\tran (I+\bar{C}_{v,t} \bar{H}_{t}\inv \bar{C}_{v,t}\tran)\inv \bar{C}_{v,t} \bar{H}_{t}\inv}],\label{ineq:super_ratio_aux_4}
\end{align}
where ineq.~\eqref{ineq:super_ratio_aux_4} holds since $\trace{\Theta_t\bar{H}_{t}\inv}$ is non-negative.  In eq.~\eqref{ineq:super_ratio_aux_4}, the second term in the sum is upper bounded as follows, using Lemma~\ref{lem:trace_low_bound_lambda_min}:
\begin{align}
&\trace{\Theta_t\bar{H}_{t}\inv \bar{C}_{v,t}\tran (I+\bar{C}_{v,t} \bar{H}_{t}\inv \bar{C}_{v,t}\tran)\inv \bar{C}_{v,t} \bar{H}_{t}\inv}= \nonumber\\
&\trace{\bar{C}_{v,t} \bar{H}_{t}\inv\Theta_t\bar{H}_{t}\inv \bar{C}_{v,t}\tran (I+\bar{C}_{v,t} \bar{H}_{t}\inv \bar{C}_{v,t}\tran)\inv}\leq \nonumber\\
&\trace{\bar{C}_{v,t} \bar{H}_{t}\inv\Theta_t\bar{H}_{t}\inv \bar{C}_{v,t}\tran} \lambda_\max[(I+\bar{C}_{v,t} \bar{H}_{t}\inv \bar{C}_{v,t}\tran)\inv]= \nonumber\\
&\trace{\bar{C}_{v,t} \bar{H}_{t}\inv\Theta_t\bar{H}_{t}\inv \bar{C}_{v,t}\tran} \lambda_\min\inv(I+\bar{C}_{v,t} \bar{H}_{t}\inv \bar{C}_{v,t}\tran)\leq \nonumber\\
&\trace{\bar{C}_{v,t} \bar{H}_{t}\inv\Theta_t\bar{H}_{t}\inv \bar{C}_{v,t}\tran} \lambda_\min\inv(I+\bar{C}_{v,t} \Sigma\att{t}{t}(\calV) \bar{C}_{v,t}\tran),\label{ineq:super_ratio_aux_5}
\end{align}
since $\lambda_\min(I+\bar{C}_{v,t} \bar{H}_{t}\inv \bar{C}_{v,t}\tran)\geq \lambda_\min(I+\bar{C}_{v,t} \Sigma\att{t}{t}(\calV) \bar{C}_{v,t}\tran)$, because  $\bar{H}_{t}\inv\succeq \Sigma\att{t}{t}(\calS'\cup \{v\})\succeq \Sigma\att{t}{t}(\calV)$; in particular, $\bar{H}_{t}\inv\succeq \Sigma\att{t}{t}(\calS'\cup \{v\})$ because $\bar{H}_{t}\preceq \bar{H}_{t}+\bar{C}_{v,t}\tran \bar{C}_{v,t}=\Sigma\att{t}{t}(\calS'\cup \{v\})\inv$.  In addition, $\Sigma\att{t}{t}(\calS'\cup\{v\})\succeq \Sigma\att{t}{t}(\calV)$ is implied from Lemma~\ref{lem:monon_t}, since $\Sigma\att{1}{1}(\calS'\cup \{v\})\succeq \Sigma\att{1}{1}(\calV)$ due to Lemma~\ref{prop:one-step_monotonicity}.
Let $l'$ to be the $\max_{t\in\until{T}, v\in \calV}\lambda_\min\inv(I+\bar{C}_{v,t} \Sigma\att{t}{t}(\calV) \bar{C}_{v,t}\tran)$.  From ineqs.~\eqref{ineq:super_ratio_aux_4} and~\eqref{ineq:super_ratio_aux_5},
\beal\label{ineq:super_ratio_aux_6}
&\sum_{t=1}^T [f_t(\calS')-f_t(\calS'\cup \{v\})]\leq
\\
&\sum_{t=1}^T [\trace{\Theta_t H_{t}\inv }+ l'\trace{\Theta_t\bar{H}_{t}\inv \bar{C}_{v,t}\tran\bar{C}_{v,t} \bar{H}_{t}\inv}].
\eeal
Consider times $t' \in \until{T}$ and $t'' \in \until{T}$ such that for any time $t \in \{1,2,\ldots,T\}$, $H_{t'}\inv  \succeq H_{t}\inv $ and $\bar{H}_{t''}\inv \bar{C}_{v,t''}\tran\bar{C}_{v,t''} \bar{H}_{t''}\inv \succeq \bar{H}_{t}\inv \bar{C}_{v,t}\tran\bar{C}_{v,t} \bar{H}_{t}\inv$, and let $\Xi=H_{t'}\inv $ and $\Phi'=\bar{H}_{t'}\inv \bar{C}_{v,t'}\tran\bar{C}_{v,t'} \bar{H}_{t'}\inv$.  From ineq.~\eqref{ineq:super_ratio_aux_6}, and Lemma~\ref{lem:traceAB_mon},
\begin{align}
&\sum_{t=1}^T [f_t(\calS')-f_t(\calS'\cup \{v\})]\leq
\nonumber\\
&\sum_{t=1}^T [\trace{\Theta_t  \Xi}+ l'\trace{ \Theta_t  \Phi'}]\leq\nonumber\\
&\trace{\Xi\sum_{t=1}^T\Theta_t }+ l'\trace{\Phi'\sum_{t=1}^T \Theta_t }\leq\nonumber \\
&(\trace{\Xi}+l'\trace{\Phi'})\lambda_\max(\sum_{t=1}^T \Theta_t).\label{ineq:super_ratio_aux_7}
\end{align}

Finally, we upper bound $\trace{\Xi}+l'\trace{\Phi'}$ in ineq.~\eqref{ineq:super_ratio_aux_7}, using Lemma~\ref{lem:trace_low_bound_lambda_min}:
\begin{align}
&\trace{\Xi}+l'\trace{\Phi'}\leq \nonumber\\
&\trace{ H_{t'}\inv}+\\
&l'\lambda_\max^2(\bar{H}_{t''}\inv)\trace{\bar{C}_{v,t''}\tran\bar{C}_{v,t''}}\leq\nonumber\\
&\trace{\Sigma\att{t'}{t'}(\emptyset)}+l'\lambda_\max^2(\Sigma\att{t''}{t''}(\emptyset))\trace{\bar{C}_{v,t''}\tran\bar{C}_{v,t''}},\label{ineq:super_ratio_aux_8}
\end{align}
where ineq.~\eqref{ineq:super_ratio_aux_8} holds because $H_{t'}\inv=\Sigma\att{t'}{t'}(\calS')\preceq \Sigma\att{t'}{t'}(\emptyset)$, and similarly, $\bar{H}_{t''}\inv\preceq \Sigma\att{t''}{t''}(\emptyset)$; in particular, $H_{t'}\inv=\Sigma\att{t'}{t'}(\calS')\preceq \Sigma\att{t'}{t'}(\emptyset)$ because of Lemma~\ref{lem:monon_t} and the fact that $\Sigma\att{1}{1}(\calS')\preceq \Sigma\att{1}{1}(\emptyset)$, which holds due to Lemma~\ref{prop:one-step_monotonicity}.  In addition, $\bar{H}_{t''}\inv\preceq \Sigma\att{t''}{t''}(\emptyset)$ since: (i)~$\bar{H}_{t''}\inv\preceq \Sigma\att{t''}{t''-1}(\calS'\cup\{v\})$, because $\bar{H}_{t''}\succeq \Sigma\inv\att{t''}{t''-1}(\calS'\cup\{v\})$; (ii)~$\Sigma\att{t''}{t''-1}(\calS'\cup\{v\})\preceq \Sigma\att{t''}{t''-1}(\emptyset)$, due to Lemma~\ref{lem:monon_t_plus_1} and the fact that $\Sigma\att{1}{1}(\calS\cup \{v\})\preceq \Sigma\att{1}{1}(\emptyset)$, which holds due to Lemma~\ref{prop:one-step_monotonicity}; and (iii)~$\Sigma\att{t''}{t''-1}(\emptyset)=\Sigma\att{t''}{t''}(\emptyset)$.
\end{proof}

We prove next the supermodularity ratio bound in ineq.~\eqref{ineq:sub_ratio_bound}.  To this end, we use the following lemma.

\begin{mylemma}\label{lem:zero_process_Sigma}
Consider for any time $t \in \until{T}$, $w_t=0$, and $A_t$ invertible. For any sensor set $\calS\subseteq \calV$, and sensor $v \in \calV$,
\begin{align*}
&\Sigma\att{t}{t-1}\inv(\calS\cup \{v\})=\\
&\Sigma\att{t}{t-1}\inv(\calS)+\\
&\sum_{k=1}^{t-1}A_{t-1}^{-\top}A_{t-2}^{-\top}\cdots A_{k+1}^{-\top}\bar{C}_{v,k+1}\tran \bar{C}_{v,k+1} A_{k+1}\inv \cdots A_{t-2}\inv A_{t-1}\inv.
\end{align*}
\end{mylemma}
\begin{proof}[Proof of Lemma~\ref{lem:zero_process_Sigma}]
From eq.~\eqref{eq:covariance_riccati} in Appendix~A,
\begin{align*}
&\Sigma\att{t}{t-1}(\calS)\inv=\\
& A_{t-1}^{-\top}(\Sigma\att{t-1}{t-2}(\calS)\inv+C_{t-1}(\calS)V_{t-1}(\calS)\inv C_{t-1}(\calS)\tran) A_{t-1}\inv,
\end{align*}
which implies
\begin{align}
& \Sigma\att{t}{t-1}(\calS)\inv+C_t(\calS)V_t(\calS)\inv C_t(\calS)\tran=\nonumber\\
& A_{t-1}^{-\top}(\Sigma\att{t-1}{t-2}(\calS)\inv+C_{t-1}(\calS)V_{t-1}(\calS)\inv C_{t-1}(\calS)\tran) A_{t-1}\inv\nonumber\\
& +C_t(\calS)V_t(\calS)\inv C_t(\calS)\tran.\label{eq:lem:zero_process}
\end{align}
Consider $\Gamma_t(\calS)=C_t(\calS)V_t(\calS)\inv C_t(\calS)\tran$, and  $X_t(\calS)=\Sigma\att{t}{t-1}(\calS)\inv+\Gamma_t(\calS)$; since for any sensor set $\calS\subseteq \calV$, $\Sigma\att{1}{0}(\calS)=\Sigma\att{1}{0}$, eq.~\eqref{eq:lem:zero_process} becomes
\begin{align}
& X_t(\calS)=\nonumber\\
&A_{t-1}^{-\top}X_{t-1}(\calS) A_{t-1}\inv+\Gamma_t(\calS)=\nonumber\\
& A_{t-1}^{-\top}A_{t-2}^{-\top}\cdots A_1^{-\top}\Sigma\att{1}{0}A_1\inv \cdots A_{t-2}\inv A_{t-1}\inv\nonumber+\\
&\sum_{k=1}^{t-1}A_{t-1}^{-\top}A_{t-2}^{-\top}\cdots A_{k+1}^{-\top}\Gamma_{k+1}(\calS) A_{k+1}\inv\cdots A_{t-2}\inv A_{t-1}\inv.\label{eq:lem:zero_process_aux_1}
\end{align}
Eq.~\eqref{eq:lem:zero_process_aux_1} implies Lemma~\ref{lem:zero_process_Sigma}, since for any time $t\in\until{T}$, $\Gamma_{t}(\calS\cup \{v\}) =\Gamma_{t}(\calS)+\Gamma_{t}(\{v\})$.
\end{proof}

\begin{proof}[Proof of Theorem~\ref{th:submod_ratio}'s supermodularity ratio bound in ineq.~\eqref{ineq:sub_ratio_bound}]
The proof follows the same steps as the proof of Theorem~\ref{th:submod_ratio} for the case where only $\sum_{t=1}^{T}\Theta_t\succ 0$.  The difference that results to the supermodularity ratio bound in ineq.~\eqref{ineq:sub_ratio_bound} is as follows:  due to Lemma~\ref{lem:zero_process_Sigma}, for any $t\in\until{T}$,  any sensor set $\calS \subseteq \calV$, and any sensor $v\in\calV$, using the Woodbury identity in Lemma~\ref{lem:woodbury}, 
\begin{align*}
& f_t(\calS)-f_t(\calS\cup\{v\})=\\
&\trace{\Theta_t\bar{\Omega}_{t}\inv \tilde{C}_{v,t}\tran (I+\tilde{C}_{v,t} \bar{\Omega}_{t}\inv \tilde{C}_{v,t}\tran)\inv \tilde{C}_{v,t} \bar{\Omega}_{t}\inv},
\end{align*}
where the matrix $\tilde{C}_{v,t}$ is such that $$\tilde{C}_{v,t}\tran \tilde{C}_{v,t}=\sum_{k=1}^{t-1}A^{-(t-k-1)\top}\bar{C}_{v}\tran \bar{C}_{v,t}A^{-(t-k-1)}.$$
\end{proof}

%\begin{mylemma}
%Let $C$ be an $p \times n$ full row rank matrix, and $B$ be an $n \times n$ positive definite matrix.
%\beq
%\lambda_\min(CBC\tran)\geq \lambda_\max\inv(C\tran (CC\tran)^{-2}C)\lambda_\min(B).
%\eeq  
%\end{mylemma}
%\begin{proof}
%Below, consider $y=C\tran x$, which implies, because $C\tran$ is full column rank, $x=(CC\tran)\inv Cy$: 
%\beal
%\lambda_\min(CBC\tran)&=\min_{x \in \mathbb{R}^p}\frac{x\tran CBC\tran x}{x\tran x}\\
%&=\min_{y \in \mathbb{R}^n}\frac{y\tran By}{y\tran  C\tran (CC\tran)^{-2}Cy}\\
%&\geq\frac{1}{\lambda_\max(C\tran (CC\tran)^{-2}C)}\min_{y \in \mathbb{R}^n}\frac{y\tran By}{y\tran y}\\
%&\geq\frac{1}{\lambda_\max(C\tran (CC\tran)^{-2}C)}\lambda_\min(B).
%\eeal
%\end{proof}

\section*{Appendix D: Proof of Theorem~\ref{th:freq}}
\label{sec:contribution}

For the proof of Theorem~\ref{th:freq}, we use the following four Lemmata~\ref{lem:it_always_holds}--\ref{lem:sum_theta}.
\begin{mylemma}\label{lem:it_always_holds}
The all-zeroes control policy $(u_1,u_2,\ldots,$ $ u_T)=(0,0,\ldots,0)$ is suboptimal for the noiseless perfect state information LQG problem in eq.~\eqref{pr:perfect_state} if and only if
\begin{equation*}
\sum_{t=1}^{T} A_1\tran \cdots A_t\tran Q_t A_t\cdots A_1\succ N_1.
\end{equation*}
\end{mylemma}
\begin{proof}[Proof of Lemma~\ref{lem:it_always_holds}]
For any initial condition $x_1\in \mathbb{R}^{n_1}$, Lemma~\ref{lem:LQG_closed} implies for the noiseless perfect state information LQG problem in eq.~\eqref{pr:perfect_state}:
\begin{equation}\label{eq:it_always_aux_1}
\min_{u_t\in \mathbb{R}^{m_t}}\sum_{t=1}^{T}\left.[x\at{t+1}\tran Q_t x\at{t+1}+u_{t}\tran R_t u_{t}]\right|_{w_t=0}=x_1\tran N_1 x_1,
\end{equation}
since $\mathbb{E}(x_1\tran N_1x_1)=x_1\tran N_1x_1$, because $x_1$ is known, and $\Sigma\att{t}{t}$ and $W_t$ are zero.
In addition, for $(u_1, u_2, \ldots, u_T)=(0,0,\ldots,0)$, the objective function in the noiseless perfect state information LQG problem in eq.~\eqref{pr:perfect_state} is 
\beal\label{eq:it_always_aux_2}
&\sum_{t=1}^{T}\left.[x\at{t+1}\tran Q_t x\at{t+1}+u_{t}\tran R_t u_{t}]\right|_{w_t=0,u_t=0}\\
&= \sum_{t=1}^{T} x\at{t+1}\tran Q_t x\at{t+1}\\ 
&=x_1\tran\sum_{t=1}^{T} A_1\tran A_2\tran \cdots A_t\tran Q_t A_tA_{t-1}\cdots A_1 x_1,
\eeal
since $x_{t+1}=A_tx_t=A_tA_{t-1}x_{t-1}=\ldots=A_tA_{t-1}\cdots A_1x_1$ when all $u_1, u_2, \ldots, u_T$ are zero.  

From eqs.~\eqref{eq:it_always_aux_1} and~\eqref{eq:it_always_aux_2}, for any non-zero $x_1 \in \mathbb{R}^{n_1}$, $$x_1\tran N_1 x_1 < x_1\tran\sum_{t=1}^{T} A_1\tran A_2\tran \cdots A_t\tran Q_t A_tA_{t-1}\cdots A_1 x_1$$ if and only if
\begin{equation*}
N_1 \prec \sum_{t=1}^{T} A_1\tran \cdots A_t\tran Q_t A_tA_{t-1}\cdots A_1.
\end{equation*}
\end{proof}

\begin{myremark}
The proof of Lemma~\ref{lem:it_always_holds} implies it always holds $N_1 \preceq \sum_{t=1}^{T} A_1\tran \cdots A_t\tran Q_t A_tA_{t-1}\cdots A_1$.
\end{myremark}

\begin{mylemma}\label{lem:theta_formula}
For any $t\in \{1,2,\ldots, T\}$, $$\Theta_t=A_t\tran S_t A_t+Q_{t-1}-S_{t-1}.$$
\end{mylemma}
\begin{proof}[Proof of Lemma~\ref{lem:theta_formula}]
Using the Woobury identity in Lemma~\ref{lem:woodbury}, and the notation in eq.~\eqref{eq:control_riccati},
\begin{align*}
N_t &= A_t\tran (S_t\inv+B_tR_t\inv B_t\tran)\inv A_t \\
&= A_t\tran (S_t - S_t B_t M_t\inv B_t\tran S_t) A_t\\
&=A_t\tran S_t A_t-\Theta_t.
\end{align*}
The latter, gives $\Theta_t=A_t\tran S_t A_t-N_t$.  In addition, from eq.~\eqref{eq:control_riccati},  $-N_t=Q_{t-1}-S_{t-1}$, since $S_t=Q_t+N_{t+1}$.
\end{proof}

\begin{mylemma}\label{lem:observability_condition}
$\sum_{t=1}^{T} A_1\tran A_2\tran \cdots A_t\tran Q_t A_tA_{t-1}\cdots A_1\succ N_1$ if and only if 
\begin{equation*}
\sum_{t=1}^{T}A\tran_{1}A\tran_2\cdots A\tran_{t-1} \Theta_t A_{t-1}A_{t-2}\cdots A_1 \succ 0.
\end{equation*}
\end{mylemma}
\begin{proof}[Proof of Lemma~\ref{lem:observability_condition}]
For $i= t-1, t-2, \ldots, 1$, we pre- and post-multiply the identity in Lemma~\ref{lem:theta_formula} with $A_i\tran$ and $A_i$, respectively:
\beal
&\Theta_t=A_t\tran S_t A_t+Q_{t-1}-S_{t-1}\Rightarrow\\
& A_{t-1}\tran\Theta_t A_{t-1}=A_{t-1}\tran A_t\tran S_t A_t A_{t-1}+A_{t-1}\tran Q_{t-1}A_{t-1}-\\
& \qquad A_{t-1}\tran S_{t-1}A_{t-1}\Rightarrow\\
& A_{t-1}\tran\Theta_t A_{t-1}=A_{t-1}\tran A_t\tran S_t A_t A_{t-1}+A_{t-1}\tran Q_{t-1}A_{t-1}-\\
& \qquad \Theta_{t-1}+Q_{t-2}-S_{t-2}\Rightarrow\\
& \Theta_{t-1}+ A_{t-1}\tran\Theta_t A_{t-1}=A_{t-1}\tran A_t\tran S_t A_t A_{t-1}+\\
&\qquad A_{t-1}\tran Q_{t-1}A_{t-1}+Q_{t-2}-S_{t-2}\Rightarrow\\
&\ldots\Rightarrow\\
& \Theta_2+ A_2\tran\Theta_3 A_2+\ldots+A_2\tran \cdots A_{t-1}\tran\Theta_t A_{t-1}\cdots A_2=\\
& A_2\tran \cdots A_t\tran S_t A_t \cdots A_2+A_2\tran \cdots A_{t-1}\tran Q_{t-1}A_{t-1}\cdots A_2+\\
&\qquad \ldots+ A_2\tran Q_2 A_2+ Q_{1}-S_{1}\Rightarrow\\
& \Theta_1+ A_1\tran\Theta_2 A_1+\ldots+A_1\tran \cdots A_{t-1}\tran\Theta_t A_{t-1}\cdots A_1=\\
& A_1\tran \cdots A_t\tran S_t A_t \cdots A_1+A_1\tran \cdots A_{t-1}\tran Q_{t-1}A_{t-1}\cdots A_1+\\
&\qquad\ldots+ A_1\tran Q_1 A_1-N_1\Rightarrow\\
&\sum_{t=1}^{T}A\tran_{1}\cdots A\tran_{t-1} \Theta_t A_{t-1}\cdots A_1 =\\
&\qquad\sum_{t=1}^{T} A_1\tran \cdots A_t\tran Q_t A_t\cdots A_1-N_1.\label{lem:obser_aux_1}
\eeal
The last equality in eq.~\eqref{lem:obser_aux_1} implies Lemma~\ref{lem:observability_condition}.
\end{proof}

\begin{mylemma}\label{lem:sum_theta}
Consider for any time $t\in \{1,2,\ldots, T\}$, $A_t$ to be invertible.
$\sum_{t=1}^{T}A\tran_{1}A\tran_2\cdots A\tran_{t-1} \Theta_t A_{t-1}A_{t-2}\cdots A_1\succ 0$ if and only if  
$$\sum_{t=1}^{T} \Theta_t \succ 0.$$
\end{mylemma}
\begin{proof}[Proof of Lemma~\ref{lem:sum_theta}] Let $U_t= A_{t-1}A_{t-2}\cdots A_1$.

We first prove that for any non-zero vector $z$, if $\sum_{t=1}^{T}A\tran_{1}A\tran_2\cdots A\tran_{t-1} \Theta_t A_{t-1}A_{t-2}\cdots A_1\succ 0$, $\sum_{t=1}^{T} z\tran\Theta_t z> 0$.  In particular, since $U_t$ is invertible, ---because for any $t\in \{1,2,\ldots, T\}$, $A_t$ is,---
\beal\label{eq:lem_sum_theta_aux_1}
\sum_{t=1}^{T} z\tran\Theta_t z&=\sum_{t=1}^{T} z\tran U_t^{-\top}U_t\tran\Theta_t U_t U_t\inv z\\
&=\sum_{t=1}^T\trace{\phi_t \phi_t\tran U_t\tran\Theta_t U_t},
\eeal
where we let $\phi_t=U_t\inv z$.  Consider a time $t'$ such that for any time $t\in \{1,2\ldots, T\}$, $\phi_{t'} \phi_{t'}\tran\preceq \phi_t \phi_t\tran$.  From eq.~\eqref{eq:lem_sum_theta_aux_1}, using Lemmata~\ref{lem:traceAB_mon} and~\ref{lem:trace_low_bound_lambda_min},
\begin{align*}
\sum_{t=1}^{T} z\tran\Theta_t z&\geq\sum_{t=1}^T\trace{\phi_{t'} \phi_{t'}\tran U_t\tran\Theta_t U_t}\\
&\geq\trace{\phi_{t'} \phi_{t'}\tran \sum_{t=1}^TU_t\tran\Theta_t U_t}\\
&\geq\trace{\phi_{t'} \phi_{t'}\tran}\lambda_\min(\sum_{t=1}^TU_t\tran\Theta_t U_t)\\
&=\|\phi_{t'}\|_2^2 \lambda_\min(\sum_{t=1}^TU_t\tran\Theta_t U_t)\\
&>0.
\end{align*}

We finally prove that for any non-zero vector $z$, if  $\sum_{t=1}^{T} \Theta_t \succ 0$, $\sum_{t=1}^{T}z A\tran_{1}\cdots A\tran_{t-1} \Theta_t A_{t-1}\cdots A_1z\succ 0$.  In particular,
\begin{align}\label{eq:lem_sum_theta_aux_2}
\sum_{t=1}^{T} z\tran U_t\tran\Theta_t U_t z&=\sum_{t=1}^T\trace{ \xi_{t}\tran \Theta_t \xi_{t}},
\end{align}
where we let $\xi_t=U_tz$.  Consider time $t'$ such that for any time $t\in \{1,2\ldots, T\}$, $\xi_{t'} \xi_{t'}\tran\preceq \xi_t \xi_t\tran$.  From eq.~\eqref{eq:lem_sum_theta_aux_1}, using Lemmata~\ref{lem:traceAB_mon} and~\ref{lem:trace_low_bound_lambda_min},
\belowdisplayskip =-12pt\begin{align*}
\sum_{t=1}^T\trace{ \xi_{t}\tran \Theta_t \xi_{t}}&\geq\trace{\xi_{t'} \xi_{t'}\tran \sum_{t=1}^T\Theta_t }\\
&\geq\trace{\xi_{t'} \xi_{t'}\tran}\lambda_\min(\sum_{t=1}^T\Theta_t)\\
&=\|\xi_{t'}\|_2^2 \lambda_\min(\sum_{t=1}^T\Theta_t )\\
&>0.
\end{align*}
\end{proof}

\begin{proof}[Proof of Theorem~\ref{th:freq}]
Theorem~\ref{th:freq} from the sequential application of Lemmata~\ref{lem:it_always_holds},~\ref{lem:observability_condition}, and~\ref{lem:sum_theta}.
\end{proof}


\section*{Appendix E: Proof of Proposition~\ref{prop:iff_for_all_zero_control}}

Proposition~\ref{prop:iff_for_all_zero_control} is Lemma~\ref{lem:it_always_holds} in Appendix~D, whose proof is also found in Appendix~D.
